# Supplementary material for: Artificial Intelligence for Literature Reviews: Opportunities and Challenges
Source: arXiv:2402.08565 source file (2024-08-06)
Supplement: Supplementary file 1 [file previousSLR_papers.tex]

% Please add the following required packages to your document preamble:
% \usepackage[table,xcdraw]{xcolor}
% Beamer presentation requires \usepackage{colortbl} instead of \usepackage[table,xcdraw]{xcolor}
\begin{table}[]
\centering
\changed{
\caption{Research manuscripts referenced as ``Previous Studies'' within the eight prior SLR surveys, employed to identify the key features for analysis. The variable `F' denotes the frequency with which a specific paper appeared in prior surveys.
 Papers deemed valid for inclusion in the current analysis are bolded and marked with Y(yes) in the `I' column.\label{tab:appendixa1}}
\footnotesize
\begin{tabular}{|p{0.5cm}|p{7cm}|l|l|p{5cm}|}
\toprule
\textbf{Id} & \textbf{Paper} & \textbf{F} & \textbf{I} & \textbf{Rationale} \\
\midrule
1  & \textbf{Online   Tools Supporting The Conduct And Reporting Of Systematic Reviews And   Systematic Maps: A Case Study On Cadima And Review Of Existing Tools}          & 3         & \textbf{Y}      & \textbf{SLR on   tools based on AI.}                                                                            \\ \hline
2  & \textbf{Software   Tools To Support Title And Abstract Screening For Systematic Reviews In   Healthcare: An Evaluation }                                               & 2         & \textbf{Y}      & \textbf{SLR on   tools based on AI.}                                                                            \\ \hline
3  & \textbf{Tools To   Support Systematic Reviews In Software Engineering: A Feature Analysis}                                                                             & 2         & \textbf{Y }     & \textbf{SLR on   tools based on AI.}                                                                            \\ \hline
4  & \textbf{Software   Tools For Literature Screening In Systematic Reviews In Biomedical Research}                                                                        & 2         & \textbf{Y}      & \textbf{SLR on   tools based on AI.}                                                                            \\ \hline
5  & Toward   Systematic Review Automation: A Practical Guide To Using Machine Learning   Tools In Research Synthesis                                              & 2         & N       & Discusses   guidelines and not a survey of AI tools.                                                   \\ \hline
6  & An Open   Source Machine Learning Framework For Efficient And Transparent Systematic   Reviews                                                                & 1         & N       & Describes   machine learning strategies not a survey of AI tools.                                      \\ \hline
7  & An R   Package To Support Article Screening For Evidence Synthesis                                                                                            & 1         & N       & It is a   tool not based on AI and not a survey of AI tools.                                           \\ \hline
8  & Experiences   Conducting Systematic Reviews From Novices’ Perspective                                                                                         & 1         & N       & Describes   user’s experience implementing SLR not a survey of AI tools.                               \\ \hline
9  & Faster   Title And Abstract Screening? Evaluating Abstrackr, A Semi-Automated Online   Screening Program For Systematic Reviewers                             & 1         & N       & Describes   experiments assessing the accuracy of the tool and not a survey of AI tools.               \\ \hline
10 & Lessons   From Applying The Systematic Literature Review Process Within The Software   Engineering Domain                                                     & 1         & N       & Describes   user’s experience implementing SLR and not a survey of AI tools.                           \\ \hline
11 & Machine   Learning For Screening Prioritization In Systematic Reviews: Comparative   Performance Of Abstrackr And Eppi-Reviewer                               & 1         & N       & Describes   experiments assessing the accuracy of the tools and not a survey of AI tools.              \\ \hline
12 & Prioritising   References For Systematic Reviews With RobotAnalyst: A User Study                                                                              & 1         & N       & Describes   experiments assessing the accuracy of the tool and not a survey of AI tools.               \\ \hline
13 & Rayyan-A   Web And Mobile App For Systematic Reviews                                                                                                          & 1         & N       & Describes   the tool and not a survey of AI tools.                                                     \\ \hline
14 & Reducing   Workload In Systematic Review Preparation Using Automated Citation   Classification                                                                & 1         & N       & Describes   the usage of machine learning in screening and not a survey of AI tools.                   \\ \hline
15 & Systematic   Literature Reviews In Software Engineering: Preliminary Results From   Interviews With Researchers                                               & 1         & N       & Describes   user’s experience implementing SLR and not a survey of AI tools.                           \\ \hline
16 & Systematic   Review Automation Technologies                                                                                                                   & 1         & N       & Describes   the automation process in SLR  and not   a survey of AI tools.                             \\ \hline
17 & Technology-Assisted   Title And Abstract Screening For Systematic Reviews: A Retrospective   Evaluation Of The Abstrackr Machine Learning Tool                & 1         & N       & Describes   experiments assessing the accuracy of the tool and not a survey of AI tools.               \\ \hline
18 & Tools To   Support Systematic Reviews In Software Engineering: A Cross-Domain Survey   Using Semi-Structured Interviews                                       & 1         & N       & Describes   user’s experience implementing SLR and not a survey of AI tools.                           \\ \hline
19 & Use Of Cost-Effectiveness   Analysis To Compare The Efficiency Of Study Identification Methods In   Systematic Reviews                                        & 1         & N       & Describes   experiments assessing the accuracy of the machine learning and not a survey   of AI tools. \\ \hline
20 & Experiences   Using Systematic Review Guidelines                                                                                                              & 1         & N       & Describes   user’s experience implementing SLR and not a survey of AI tools.                           \\ \hline
21 & Identification   Of Slr Tool Needs—Results Of A Community Workshop                                                                                            & 1         & N       & Describes   user’s needs on the automation of SLR and not a survey of AI tools.                        \\ \hline
22 & Making   Progress With The Automation Of Systematic Reviews: Principles Of The   International Collaboration For The Automation Of Systematic Reviews (Icasr) & 1         & N       & Describes   user’s needs on the automation of SLR and not a survey of AI tools.                        \\ \hline
23 & Performance   And Usability Of Machine Learning For Screening In Systematic Reviews: A   Comparative Evaluation Of Three Tools                                & 1         & N       & Describes   experiments assessing the accuracy of the tool and not a survey of AI tools.         \\
\bottomrule
\end{tabular}
}
\end{table}


\begin{table}[]
\centering
\changed{
\caption{Seed Papers of the 3 prior SLR surveys that employed Snowballing Search. The variable `F' denotes the frequency with which a specific paper appeared in prior surveys. Papers deemed valid for inclusion in the current analysis are bolded and marked with Y(yes) in the `I' column.\label{tab:appendixa2}}
\footnotesize
\begin{tabular}{|p{0.5cm}|p{8cm}|l|l|p{4cm}|}
\toprule
\textbf{Id} & \textbf{Paper} & \textbf{F} & \textbf{I} & \textbf{Rationale} \\
\midrule
1  & \textbf{Rayyan-A   Web And Mobile App For Systematic Reviews}                                                                                                          & 2         & \textbf{Y}        & \textbf{Describes   a tool based on AI}.                                                        \\ \hline
2  & \textbf{Fast2 :   An Intelligent Assistant For Finding Relevant Papers}                                                                                                & 1         & \textbf{Y}        & \textbf{Describes   a tool based on AI}.                                                        \\ \hline
3  & Tools To Support Systematic Literature   Reviews In Software Engineering: A Mapping Study                                                                     & 1         & N       & It is a survey   about SLR.                                                            \\ \hline
4  & A   Critical Analysis Of Studies That Address The Use Of Text Mining For Citation   Screening In Systematic Reviews                                           & 1         & N       & Describes   experiments assessing the accuracy of the tools not their functionalities. \\ \hline
5  & A Visual   Analysis Approach To Validate The Selection Review Of Primary Studies In   Systematic Reviews                                                      & 1         & N       & Describes   visualization techniques to improve the screening process.                 \\ \hline
6  & An Open   Source Machine Learning Framework For Efficient And Transparent Systematic   Reviews                                                                & 1         & N       & Describes   experiments employing the tool.                                            \\ \hline
7  & Conducting   Systematic Literature Reviews And Systematic Mapping Studies                                                                                     & 1         & N       & Describes   experiments employing the tool.                                            \\ \hline
8  & Deploying   An Interactive Machine Learning System In An Evidence-Based Practice Center:   Abstrackr                                                          & 1         & N       & Describes   experiments employing the tool.                                            \\ \hline
9  & Faster   Title And Abstract Screening? Evaluating Abstrackr, A Semi-Automated Online   Screening Program For Systematic Reviewers                             & 1         & N       & Describes   experiments employing the tool.                                            \\ \hline
10 & Improvements   In The Start Tool To Better Support The Systematic Review Process                                                                              & 1         & N       & Describes   a tool not based on AI.                                                    \\ \hline
11 & Prioritising   References For Systematic Reviews With RobotAnalyst: A User Study                                                                              & 1         & N       & Describes   experiments employing the tool.                                            \\ \hline
12 & Reducing   Workload In Systematic Review Preparation Using Automated Citation   Classification                                                                & 1         & N       & Describes   experiments employing the tool.                                            \\ \hline
13 & Revtools:   An R Package To Support Article Screening For Evidence Synthesis                                                                                  & 1         & N       & Describes   a tool not based on AI.                                                    \\ \hline
14 & Semi-Automatic   Selection Of Primary Studies In Systematic Literature Reviews: Is It   Reasonable?                                                           & 1         & N       & Describes   experiments employing the tool.                                            \\ \hline
15 & Slr-Tool   - A Tool For Performing Systematic Literature Reviews                                                                                              & 1         & N       & Describes   a tool not based on AI.                                                    \\ \hline
16 & Slurp: A   Tool To Help Large Complex Systematic Literature Reviews Deliver Valid And   Rigorous Results                                                      & 1         & N       & Describes   a tool not based on AI.                                                    \\ \hline
17 & Systematic   Review Automation Technologies                                                                                                                   & 1         & N       & Describes   the automation process in SLR                                              \\ \hline
18 & Technology-Assisted   Title And Abstract Screening For Systematic Reviews: A Retrospective   Evaluation Of The Abstrackr Machine Learning Tool                & 1         & N       & Describes   experiments employing the tool.                                            \\ \hline
19 & Text And   Data Mining For Researchers: Investigating Trends To Update Collaboration   Services                                                               & 1         & N       & Describes   the usage of text mining in the automation of SLR.                         \\ \hline
20 & Tool   Support For Systematic Reviews In Software Engineering                                                                                                 & 1         & N       & It is a   survey about SLR.                                                            \\ \hline
21 & Toward   Systematic Review Automation: A Practical Guide To Using Machine Learning   Tools In Research Synthesis                                              & 1         & N       & Discusses   guidelines for using machine learning.                                     \\ \hline
22 & Use Of   Cost-Effectiveness Analysis To Compare The Efficiency Of Study Identification   Methods In Systematic Reviews                                        & 1         & N       & Describes   experiments employing the tool.                                            \\ \hline
23 & Using   Text Mining For Study Identification In Systematic Reviews: A Systematic   Review Of Current Approaches                                               & 1         & N       & Describes   the usage of text mining in the automation of SLR.                         \\ \hline
24 & Using The   Scas Strategy To Perform The Initial Selection Of Studies In Systematic   Reviews: An Experimental Study                                          & 1         & N       & Describes   experiments employing the tool.                                            \\ \hline
25 & A   Systematic Review Of Systematic Review Process Research In Software   Engineering                                                                         & 1         & N       & It is a survey about SLR \tocheck{(It is a survey about how to conduct SLRs.)??}.                                                            \\ \hline
26 & How To   Read Less: Better Machine Assisted Reading Methods For Systematic Literature   Reviews                                                               & 1         & N       & Describes   experiments employing the tool.                                            \\ \hline
27 & Making   Progress With The Automation Of Systematic Reviews: Principles Of The   International Collaboration For The Automation Of Systematic Reviews (Icasr) & 1         & N       & Describes   user’s needs on the automation of SLR.   \\
\bottomrule
\end{tabular}
}
\end{table}
