# Supplementary material for: Artificial Intelligence for Literature Reviews: Opportunities and Challenges
Source: arXiv:2402.08565 source file (2024-08-06)
Supplement: Supplementary file 2 [file prisma_checklist.tex]

% Please add the following required packages to your document preamble:
% \usepackage{multirow}
% \usepackage[table,xcdraw]{xcolor}
% Beamer presentation requires \usepackage{colortbl} instead of \usepackage[table,xcdraw]{xcolor}

\color{black}

\begin{longtable}{|p{2cm}|p{0.6cm}|p{9cm}|p{2cm}|}
% \begin{tabular}{|p{2cm}|p{1cm}|p{10cm}|p{2cm}|}
\rowcolor[HTML]{63639A} 
\textbf{Section and Topic  }                              & \textbf{Item \#} & \textbf{Checklist item }                                                                                                                                                                                                                                                                                              & \textbf{Location where item is reported} \\ \hline
\rowcolor[HTML]{FFFFCC} 
\multicolumn{3}{|l|}{\cellcolor[HTML]{FFFFCC}\textbf{TITLE}}                                                                                                                                                                                                                                                                                                                         &                                 \\ \hline
Title                                            & 1       & Identify   the report as a systematic review.                                                                                                                                                                                                                                                                & 1                               \\ \hline
\rowcolor[HTML]{FFFFCC} 
\multicolumn{3}{|l|}{\cellcolor[HTML]{FFFFCC}\textbf{ABSTRACT}}                                                                                                                                                                                                                                                                                                                      &                                 \\ \hline
Abstract                                         & 2       & See   the PRISMA 2020 for Abstracts checklist.                                                                                                                                                                                                                                                               & 1                               \\ \hline
\rowcolor[HTML]{FFFFCC} 
\multicolumn{3}{|l|}{\cellcolor[HTML]{FFFFCC}\textbf{INTRODUCTION}}                                                                                                                                                                                                                                                                                                                  &                                 \\ \hline
Rationale                                        & 3       & Describe   the rationale for the review in the context of existing knowledge.                                                                                                                                                                                                                                & 2                               \\ \hline
Objectives                                       & 4       & Provide   an explicit statement of the objective(s) or question(s) the review   addresses.                                                                                                                                                                                                                   & 2                               \\ \hline
\rowcolor[HTML]{FFFFCC} 
\multicolumn{3}{|l|}{\cellcolor[HTML]{FFFFCC}\textbf{METHODS}}                                                                                                                                                                                                                                                                                                                       &                                 \\ \hline
Eligibility   criteria                           & 5       & Specify   the inclusion and exclusion criteria for the review and how studies were   grouped for the syntheses.                                                                                                                                                                                              & 5                               \\ \hline
Information   sources                            & 6       & Specify   all databases, registers, websites, organisations, reference lists and other   sources searched or consulted to identify studies. Specify the date when each   source was last searched or consulted.                                                                                              & 4,6,7, Appendix A               \\ \hline
Search   strategy                                & 7       & Present   the full search strategies for all databases, registers and websites,   including any filters and limits used.                                                                                                                                                                                     & 5,6,7                           \\ \hline
Selection   process                              & 8       & Specify   the methods used to decide whether a study met the inclusion criteria of the   review, including how many reviewers screened each record and each report   retrieved, whether they worked independently, and if applicable, details of   automation tools used in the process.                     & 6                               \\ \hline
Data   collection process                        & 9       & Specify   the methods used to collect data from reports, including how many reviewers   collected data from each report, whether they worked independently, any   processes for obtaining or confirming data from study investigators, and if   applicable, details of automation tools used in the process. & 6,23                            \\ \hline
                                                 & 10a     & List   and define all outcomes for which data were sought. Specify whether all   results that were compatible with each outcome domain in each study were   sought (e.g. for all measures, time points, analyses), and if not, the   methods used to decide which results to collect.                        & N/A                             \\ \cliness{2-4} 
\multirow{-2}{2cm}{Data   items}                   & 10b     & List   and define all other variables for which data were sought (e.g. participant   and intervention characteristics, funding sources). Describe any assumptions   made about any missing or unclear information.                                                                                           & 8,9,10,11                       \\ \hline
Study   risk of bias assessment                  & 11      & Specify   the methods used to assess risk of bias in the included studies, including   details of the tool(s) used, how many reviewers assessed each study and   whether they worked independently, and if applicable, details of automation   tools used in the process.                                    & 6                               \\ \hline
Effect   measures                                & 12      & Specify   for each outcome the effect measure(s) (e.g. risk ratio, mean difference)   used in the synthesis or presentation of results.                                                                                                                                                                      & N/A                             \\ \hline
                                                 & 13a     & Describe   the processes used to decide which studies were eligible for each synthesis   (e.g. tabulating the study intervention characteristics and comparing against   the planned groups for each synthesis (item \#5)).                                                                                  & 23                              \\ \cliness{2-4} 
                                                 & 13b     & Describe   any methods required to prepare the data for presentation or synthesis, such   as handling of missing summary statistics, or data conversions.                                                                                                                                                    & N/A                             \\ \cliness{2-4}
                                                 & 13c     & Describe   any methods used to tabulate or visually display results of individual   studies and syntheses.                                                                                                                                                                                                   & N/A                             \\ \cliness{2-4}
                                                 & 13d     & Describe   any methods used to synthesize results and provide a rationale for the   choice(s). If meta-analysis was performed, describe the model(s), method(s)   to identify the presence and extent of statistical heterogeneity, and   software package(s) used.                                          & N/A                             \\ \cliness{2-4}
                                                 & 13e     & Describe   any methods used to explore possible causes of heterogeneity among study   results (e.g. subgroup analysis, meta-regression).                                                                                                                                                                     & N/A                             \\ \cliness{2-4}
\multirow{-6}{2cm}{Synthesis   methods}            & 13f     & Describe   any sensitivity analyses conducted to assess robustness of the synthesized   results.                                                                                                                                                                                                             & N/A                             \\ \hline
Reporting   bias assessment                      & 14      & Describe   any methods used to assess risk of bias due to missing results in a synthesis   (arising from reporting biases).                                                                                                                                                                                  & 21, Interview                   \\ \hline
Certainty   assessment                           & 15      & Describe   any methods used to assess certainty (or confidence) in the body of evidence   for an outcome.                                                                                                                                                                                                    & NA                              \\ \hline
\rowcolor[HTML]{FFFFCC} 
\multicolumn{3}{|l|}{\cellcolor[HTML]{FFFFCC}\textbf{RESULTS}}                                                                                                                                                                                                                                                                                                                       &                                 \\ \hline
                                                 & 16a     & Describe   the results of the search and selection process, from the number of records identified   in the search to the number of studies included in the review, ideally using   a flow diagram.                                                                                                           & Fig 1                           \\ \cliness{2-4}
\multirow{-2}{2cm}{Study   selection}              & 16b     & Cite   studies that might appear to meet the inclusion criteria, but which were   excluded, and explain why they were excluded.                                                                                                                                                                              & 7                               \\ \hline
Study   characteristics                          & 17      & Cite   each included study and present its characteristics.                                                                                                                                                                                                                                                  & Appendix C                      \\ \hline
Risk   of bias in studies                        & 18      & Present   assessments of risk of bias for each included study.                                                                                                                                                                                                                                               & N/A                             \\ \hline
Results   of individual studies                  & 19      & For   all outcomes, present, for each study: (a) summary statistics for each group   (where appropriate) and (b) an effect estimates and its precision (e.g.   confidence/credible interval), ideally using structured tables or plots.                                                                      & Appendix C                      \\ \hline
                                                 & 20a     & For   each synthesis, briefly summarise the characteristics and risk of bias among   contributing studies.                                                                                                                                                                                                   & 12-21                           \\ \cliness{2-4}
                                                 & 20b     & Present   results of all statistical syntheses conducted. If meta-analysis was done,   present for each the summary estimate and its precision (e.g.   confidence/credible interval) and measures of statistical heterogeneity. If   comparing groups, describe the direction of the effect.                 & Table 5                         \\ \cliness{2-4}
                                                 & 20c     & Present   results of all investigations of possible causes of heterogeneity among study   results.                                                                                                                                                                                                           & N/A                             \\ \cliness{2-4}
\multirow{-4}{2cm}{Results   of syntheses}         & 20d     & Present   results of all sensitivity analyses conducted to assess the robustness of the   synthesized results.                                                                                                                                                                                               & N/A                             \\ \hline
Reporting   biases                               & 21      & Present   assessments of risk of bias due to missing results (arising from reporting   biases) for each synthesis assessed.                                                                                                                                                                                  & N/A                             \\ \hline
Certainty   of evidence                          & 22      & Present   assessments of certainty (or confidence) in the body of evidence for each   outcome assessed.                                                                                                                                                                                                      & N/A                             \\ \hline
\rowcolor[HTML]{FFFFCC} 
\multicolumn{3}{|l|}{\cellcolor[HTML]{FFFFCC}\textbf{DISCUSSION}}                                                                                                                                                                                                                                                                                                                    &                                 \\ \hline
                                                 & 23a     & Provide   a general interpretation of the results in the context of other evidence.                                                                                                                                                                                                                          & 24-28                           \\ \cliness{2-4}
                                                 & 23b     & Discuss   any limitations of the evidence included in the review.                                                                                                                                                                                                                                            & 21-24                           \\ \cliness{2-4}
                                                 & 23c     & Discuss   any limitations of the review processes used.                                                                                                                                                                                                                                                      & 21-24                           \\ \cliness{2-4}
\multirow{-4}{2cm}{Discussion}                     & 23d     & Discuss   implications of the results for practice, policy, and future research.                                                                                                                                                                                                                             & 28-31                           \\ \hline
\rowcolor[HTML]{FFFFCC} 
\multicolumn{3}{|l|}{\cellcolor[HTML]{FFFFCC}OTHER   INFORMATION}                                                                                                                                                                                                                                                                                                           &                                 \\ \hline
                                                 & 24a     & Provide   registration information for the review, including register name and   registration number, or state that the review was not registered.                                                                                                                                                           & Not registered                  \\ \cliness{2-4}
                                                 & 24b     & Indicate   where the review protocol can be accessed, or state that a protocol was not   prepared.                                                                                                                                                                                                           & Pending                         \\ \cliness{2-4}
\multirow{-3}{2cm}{Registration and protocol}    & 24c     & Describe   and explain any amendments to information provided at registration or in the   protocol.                                                                                                                                                                                                          & N/A                             \\ \hline
Support                                          & 25      & Describe   sources of financial or non-financial support for the review, and the role of   the funders or sponsors in the review.                                                                                                                                                                            & N/A                             \\ \hline
Competing   interests                            & 26      & Declare   any competing interests of review authors.                                                                                                                                                                                                                                                         & Pending                         \\ \hline
Availability   of data, code and other materials & 27      & Report   which of the following are publicly available and where they can be found:   template data collection forms; data extracted from included studies; data   used for all analyses; analytic code; any other materials used in the review.                                                             & Appendix A,B,C, Script         \\ \hline
% \end{tabular}
\end{longtable}
